# Supplementary material for: Model checking memoryful linear-time logics over one-counter automata
Source: arXiv:0810.5517 source file (2010-01-18)
Supplement: Supplementary file 1 [file appendix.tex]

%% 
%% \section{Proof of Lemma~\ref{lemma-purification}}
%% \label{section-proof-purification-lemma}
%% 
%% \input{proof-purification-lemma}
%% 

\section{Proofs in  Section~\ref{section-properties}}
\label{section-proofs-section-properties}

\subsection{Proof of Proposition~\ref{proposition-pspace-hardness}}

\input{proof-pspace-hardness}

%% 
%% Ste 051007
%% 
%% \subsection{Proof of Lemma~\ref{lemma-between-zero-tests}}
%% 
%% \input{proof-lemma-between-zero-tests}
%% 
%% 

\subsection{Proof of Lemma~\ref{lemma-KKK}}

\input{proof-lemma-KKK}

\section{Proofs in Section~\ref{section-pspace}}
\label{section-proofs-section-pspace}

\subsection{Proof of Lemma~\ref{lemma-bound-context}}

(I) Ad absurdum, suppose that $j-i > K_1+K_1 K_2$. First, observe that $n_i < K_1$. 
Let $m$ be the minimal value in $\set{n_{K_1}, \ldots, n_{K_1+K_2-1}}$.
For all $l \geq K_1 + K_1 K_2$, we have $n_l \geq m + K_1 K_3 \geq K_1 K_3 > K_1$. Since 
$j \geq K_1 + K_1 K_2$, we deduce that $n_j > K_1$, 
which is in contradiction with  $n_i=n_j$.

(II) Ad absurdum, suppose that $(j-i) > K_2^2$. Remark that from a position $l \geq K_1$, we have for all $l' >l$, $n_{l'} \geq n_l -K_2/2$, in fact performing $K_2$ transitions after a position greater than $K_1$ amounts to add $K_3$ to every counter value. Consequently we can deduce that $n_j \geq n_{i+K_2^2} - K_2/2$. Since $n_{i+K_2^2}=n_{i}+K_2 K_3$, we conclude that 
$n_j \geq n_{i}+K_2 K_3 - K_2/2 \geq n_{i}+K_2- K_2/2 > n_i$, which leads to 
a contradiction. 

\subsection{Proof of Lemma~\ref{lemma-polynomial}}

 First, suppose that $K_3 = 0$. The run 
 $\arun_{\aautomaton}^{\omega}$ is of the form
 $$\pair{\aloc_0}{n_0} \cdots \pair{\aloc_{K_1-1}}{n_{K_1-1}}
 (\pair{\aloc_{K_1}}{n_{K_1}} \cdots \pair{\aloc_{K_1+
     K_2-1}}{n_{K_1+K_2-1}})^{\omega}.
$$
It is easy to see that for all $i \in \Nat$ and $m \not \in 
\set{n_0, \ldots, n_{K_1 + K_2 -1}}$, ${\rm pos}_{\aautomaton}(i,m) = \emptyset$. 
Moreover, 
\begin{itemize}
\itemsep 0 cm
\item for all $i,i' \geq K_1$ such that $i \equiv_{K_2} i'$ and register values
      $m \in \Nat$,
      we have ${\rm pos}_{\aautomaton}(i,m) =  {\rm pos}_{\aautomaton}(i',m)$,,
\item for every $i \leq K_1 + K_2 -1$,
      $$
\set{{\rm pos}_{\aautomaton}(i,m) \subseteq \Nat:  \ m \in \set{n_0, \ldots,n_i}}
      $$
      has cardinality at most $i + 1$.
\end{itemize}
%% Arn 310807
%%
%%Consequently, $\regvalues$ has cardinalities at most $(K_1 + K_2)^2 + K_2 + 1$. \\
Consequently, from the first point, we have
 $\regvalues=\set{{\rm pos}_{\aautomaton}(i,m): i \in \set{0, \ldots, K_1+K_2-1}, m \in \set{n_0, \ldots,n_i}} \cup \set{\emptyset}$  
whereas from  the second point, we get that its cardinality is at most $(K_1 + K_2)^2 + 1$.\\ 

Second, suppose that $K_3 > 0$ (and therefore $K_2 \leq \length{\locs}$). 
 The run 
 $\arun_{\aautomaton}^{\omega}$ is of the form below
$$\pair{\aloc_0}{n_0} \cdots \pair{\aloc_{K_1}}{n_{K_1}}
\cdots \pair{\aloc_{K_1+K_2}}{n_{K_1} + K_3} \cdots 
 \pair{\aloc_{K_1+2K_2}}{n_{K_1} + 2K_3} \cdots 
$$
The set $\set{n_j: j \geq 0}$ is therefore infinite
and $\aloc_{K1} = \aloc_{K_1 + K_2} = \aloc_{K_1 + 2K_2} = \ldots$. From lemma \ref{lemma-bound-context}, we deduce the following observations that will allow us to get the polynomial cardinality for $\regvalues$.
\begin{enumerate}
\itemsep 0 cm
\item The set $\set{{\rm pos}_{\aautomaton}(i,m): 0 \leq i \leq 
      K_1 + K_2^2, \ m \in \set{n_0, \ldots,n_i}}$ has at most $(1 + K_1 +  K_2^2)^2$ elements,
      which is polynomial in $\length{\locs}$.
\item For every $i \geq K_1 + K_2^2$, if $m \not \in \set{0, \ldots,K_1-1} \cup \set{n_{(i - K_2^2) + 1 }, \ldots, n_i}$,
      then ${\rm pos}_{\aautomaton}(i,m)$ is the empty set.
      %
      %Arn 040907
      %Indeed, performing $K_2$ transitions after a position greater than $K_1$ amounts to add $K_3 > 0$ to every counter value.
      %Hence, $\set{{\rm pos}_{\aautomaton}(i,m): \ m \in \set{n_0,
      %    \ldots,n_i}}$ has cardinality at most $K_2^2 + 1$.
      Hence, $\set{{\rm pos}_{\aautomaton}(i,m): \ m \in \set{n_0,
          \ldots,n_i}}$ has cardinality at most $K_2^2 + K_1 + 1$.
\item For all $i \geq K_1 + K_2^2$ and $m \in \set{n_{(i - K_2^2) + 1 }, \ldots, n_i}$,
      ${\rm pos}_{\aautomaton}(i+ K_2, m + K_3) = {\rm pos}_{\aautomaton}(i,m)$.
      Hence, for all $i,i' \geq K_1 + K_2^2$ such that $i \equiv_{K_2} i'$, 
      $$
      \set{{\rm pos}_{\aautomaton}(i,m): \ m \in \set{n_0, \ldots,n_i}} =
      \set{{\rm pos}_{\aautomaton}(i',m): \ m \in \set{n_0, \ldots,n_{i'}}}.
      $$
\end{enumerate}

\subsection{Proof of Lemma~\ref{lemma-two-in-one}}

(I) The proof is done by recurrence on $j$. First suppose that $j=1$. 
    The only point to check is that  $\aloc_{i+1}=\aloc_{i'+1}$, which is a simple consequence
of the determinism of $\aautomaton$. Indeed,  if there is only an incrementing transition from $\aloc_i$,
 then we get straightforwardly $q_{i+1}=q_{i'+1}$. Otherwise, if there are 
two transitions from $\aloc_i$, then  one is a decrementation and the other one is a zero-test.
The induction step is shown in a similar fashion. 

(II) Suppose $\pair{i}{\aregval} \equiv \pair{i'}{\aregval'}$.
The proof is by structural induction on $\aformulabis$.
\begin{itemize}
\itemsep 0 cm 
\item Case  $\aformulabis=q$: Since by definition $i \equiv i'$, we have that $q_i=q_{i'}$ and consequently $q_i=q$ iff $q_{i'}=q$.
\item Case  $\aformulabis=\uparrow_r $:
Since $n_i=v(r)$ iff $n_{i'}=v'(r)$, we have that $\arun_{\aautomaton}^{\omega}, i \models_{\aregval} \uparrow_r  $ iff
$\arun_{\aautomaton}^{\omega}, i' \models_{\aregval'} \uparrow_r $.
\item Case  $\aformulabis=\mynext \aformula$: Since $\pair{i}{\aregval} \equiv \pair{i'}{\aregval'}$, 
from Lemma~\ref{lemma-two-in-one}(I), 
we deduce that $\pair{i+1}{\aregval} \equiv \pair{i+1'}{\aregval'}$ and 
by (IH) we obtain  $\arun_{\aautomaton}^{\omega}, i+1 \models_{\aregval} \aformulabis$ iff
$\arun_{\aautomaton}^{\omega}, i'+1 \models_{\aregval'} \aformulabis$.
\item Case  $\aformulabis = \aformula_1 \until \aformula_2$: 
Suppose that there exists $j \geq 0$ such that $\arun_{\aautomaton}^{\omega}, i+j \models_{\aregval} \aformula_2$ and for all $0 \leq j' < j$, $\arun_{\aautomaton}^{\omega}, i+j' \models_{\aregval} \aformula_1$. 
Using Lemma~\ref{lemma-two-in-one}(I) and (IH),  
we deduce that $\arun_{\aautomaton}^{\omega}, i'+j \models_{\aregval} \aformula_2$ and for all $0 \leq j' < j$, $\arun_{\aautomaton}^{\omega}, i'+j' \models_{\aregval} \aformula_1$.
\item Case  $\aformulabis=\downarrow_r \aformula$:
We observe that if  $\pair{i}{\aregval} \equiv \pair{i'}{\aregval'}$ then $\pair{i}{\aregval[r \mapsto n_i]} \equiv 
\pair{i'}{\aregval'[r \mapsto n_i]}$. This is due to the fact that for 
$\alpha \geq 0,$ if $n_{i+a}=n_i$, then $n_i'=n_{i'+\alpha}$ (since $i \equiv i'$). 
By (IH), we get the desired result.
\end{itemize}

\subsection{Proof of Lemma~\ref{lemma-next}}

Let $\pair{i'}{pos'}=[\pair{i}{\aregval}]$, $\pair{i''}{pos''}=[\pair{i+1}{\aregval}]$ and $\pair{j}{pos}=\movnext([\pair{i}{\aregval}])$.

First, we will show that $pos''=pos$. Suppose $K_3=0$, then we have that $pos=pos'$. 
Since for all $r \in \set{1, \ldots, N}$, $pos'(r)=v(r)=pos''(r)$, we deduce that $pos''=pos$. 
Now consider the case $K_3>0$. Then for $r \in  \set{1, \ldots , N}$, 
$pos(r)=\set{\alpha-1 : \alpha \in pos'(r) , \alpha >0}$. 
Furthermore $pos'(r)={\rm pos}_{\aautomaton}(i,\aregval(r))=\set{l \in \Nat : n_{i+l}=\aregval(r)}$. 
Let $l \in pos''(r)$ such that $l \geq 0$. 
Then $n_{i+1+l-1}=n_{i+l}=\aregval(r)$ and we can deduce that 
$l-1 \in {\rm pos}_{\aautomaton}(i+1,\aregval(r))=pos''(r)$. 
Now we suppose  that $l \in pos''(r)$. Hence, $n_{i+1+l}=\aregval(r)$. 
If we denote $l+1$ by $l'$, then $l' \in pos'(r)$ and since $l=l'-1$, we obtain that $l \in pos(r)$.

We will now show that $i''=j$. First, we suppose that $i+1 \leq K_1+K_2-1$ then $i''=i+1=j$. Second, we suppose that $i+1 > K_1+K_2-1$. So we have that $i'' \equiv_{K_2} i + 1 \equiv_{K_2} j $ and since we have that $i'',j \in \set{K_1, \ldots K_1 + K_2 - 1}$, we deduce that $i''=j$.

%% Arn 081007
%%\subsection{Proof of Lemma~\ref{lemma-until}}
%%
%%
%% \input{proof-lemma-until}

\section{Proof sketch  of Theorem~\ref{theorem-undecidability-weakly}}
\label{section-proof-theorem-undecidability-weakly}

\input{proof-theorem-undecidability-weakly}
